# Supplementary material for: Editing Personality for Large Language Models
Source: arXiv:2310.02168 source file (2024-09-01)
Supplement: Supplementary file 1 [file appendix.tex]

\begin{figure*}[ht]
    \centering
    \includegraphics[width=0.95\textwidth]{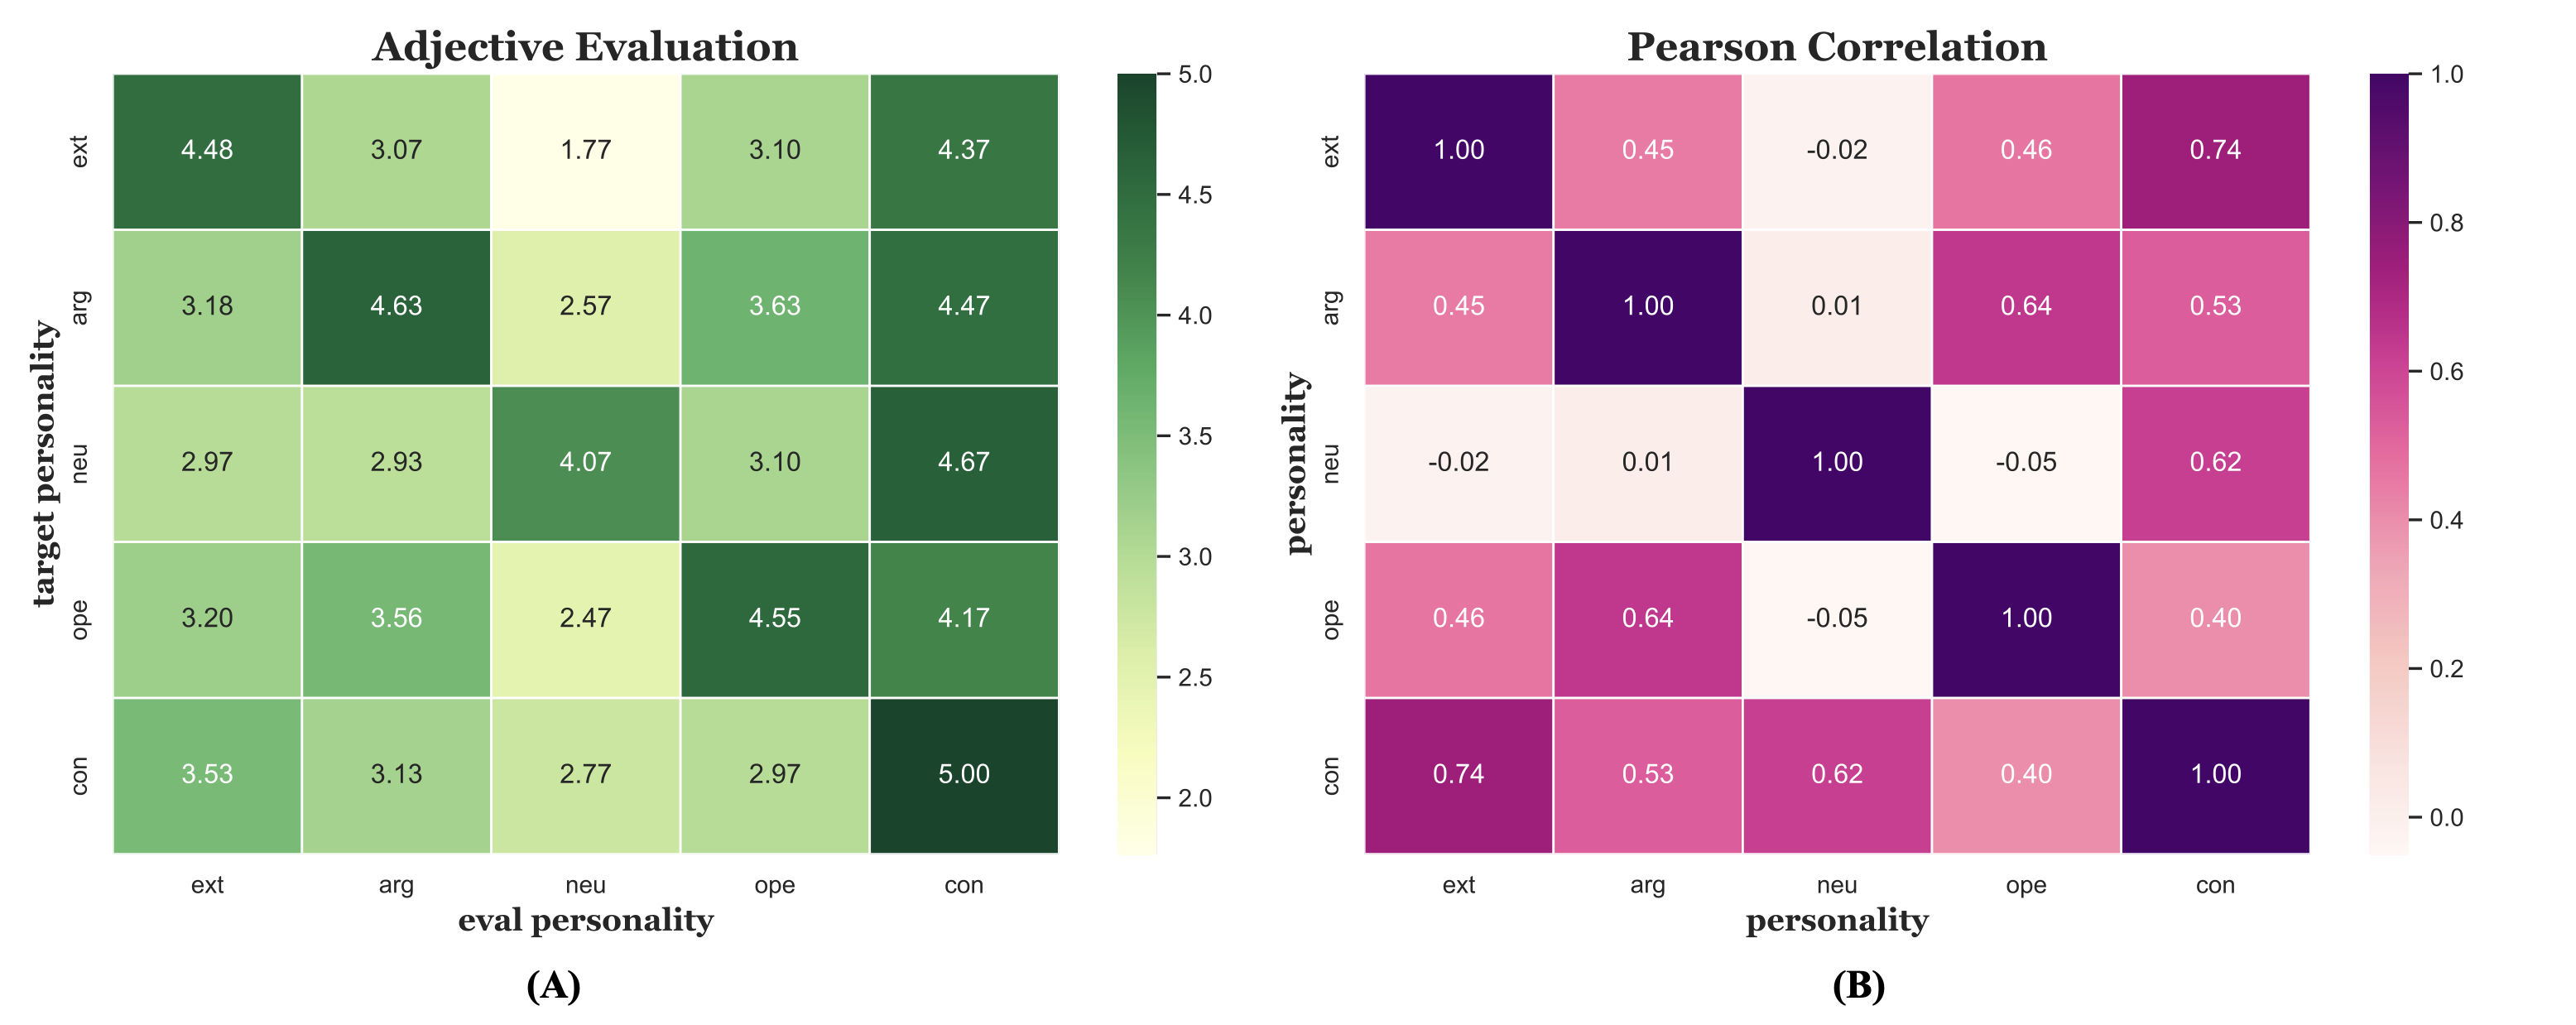}
    \caption{The Personality Adjective Evaluation~\textbf{(A)} and Pearson Correlation(B) of the personality analysis in 30 testing cases.}
    \label{fig:heatmaps}
\end{figure*}

\section{Appendix}

\subsection{Reproducibility Statement}

%Codes and datasets are in the supplementary materials and will be released on Github.
% Codes and datasets will be released at \url{https://github.com/zjunlp/EasyEdit}.
The corresponding calculation formulas for our experimental metrics can be found in the Appendix~\ref{appendix:metric}.
Additionally, we have provided the specific code for metric computation in the supplementary experimental materials. We also furnish the code used to train the classifier for our metrics as well as the hyperparameters in Appendix~\ref{appendix:classifier}.
Subsequently, we intend to publicly release the parameters of our classifier and the trained weights for edited models in the future.

\subsection{Data Construction}\label{sec:appendix_data_construction}

\subsubsection{Personality Selection}\label{sec:personality_selection}

To precisely select personalities for expressing viewpoints, we initially generate data for 30 topics across five personality types. After obtaining the verified textual data, we evaluate the PAE score for each of the five personality texts across every topic. Specifically, for a given topic $t$, we have 5 pre-generated opinion texts, denoted as $y_1, y_2, y_3, y_4, y_5$, corresponding to the five personality types. We then compute the PAE score for each personality text against each eval personality, e.g. $\mathrm{pae}(y_1, p_1)$, and subsequently determine the average across all 30 topics.

From Figure~\ref{fig:heatmaps} \textbf{(A)}, it can be observed that the generated texts corresponding to \textsc{Extraversion}, \textsc{Agreeableness}, \textsc{Neuroticsim}, and \textsc{Openness} often exhibit traits of the \textsc{Conscientiousness} personality. In some instances, the scores even surpass those of the intended personality. This suggests that \textsc{Conscientiousness} lacks distinctiveness in the editing task and should be excluded. The differentiation between \textsc{Extraversion} and \textsc{Neuroticsim} personalities compared to the remaining \textsc{Agreeableness} and \textsc{Openness} is also apparent.
We also calculate the Pearson correlation scores between the PAE scores of our five personalities, as illustrated in Figure~\ref{fig:heatmaps} \textbf{(B)}. Notably, a certain degree of association is discernible between \textsc{Openness} and \textsc{Agreeableness}. To emphasize distinctiveness, we manually analyze dozens of cases. We discover that, comparatively, the viewpoints expressed by the Agreeableness personality are more distinct from those of the \textsc{Openness} personality, especially when compared against \textsc{Extraversion} and \textsc{Neuroticsim}. As such, we finally select \textsc{Extraversion}, \textsc{Neuroticsim}, and \textsc{Agreeableness}.

\input{tab/statistic_table}

\subsubsection{Topic Selection}\label{sec:topic_selection}

During the process of topic selection, we use wikipedia view counts as an indicator of popularity.
Specifically, we filter the topics viewed over 5,000 times from the entities available in the ConvSent dataset~\cite{serac}, comprising a total of 15,989 entries gathered from zsRE and GPT-3,
% which are assembled from zsRE~\cite{DBLP:conf/conll/LevySCZ17,DBLP:conf/emnlp/CaoAT21} and GPT-3~\cite{gpt3}. 
as our candidate pool for potential selection. 
After eliminating the unpopular topics, we sample according to the topic distribution, resulting in our final selection of 2,000 topics. The distribution of all topics and selected topics is shown in Figure~\ref{topic_selection}.
% we posit that GPT-4 is capable of generating higher quality data—more accurately reflecting the selected personality facets—for topics associated with higher popularity.

\begin{table*}[t!]
\centering
\scalebox{0.8}{
\begin{tabular}{l|c|c}
    \toprule
    \textbf{Personality} & \textbf{Facets} & \textbf{Adjectives} \\
    \midrule
    \multirow{2}{*}{\textsc{Extraversion}} & gregariousness, excitement-seeking, activity Level & friendly, talkative, assertive \\
    & cheerfulness, assertive, friendliness & cheerful, adventurous and daring \\
    \midrule
    \multirow{2}{*}{\textsc{Neuroticsim}} & anger, anxiety, self-consciousness & depressed, impulsive, discontented \\
    & depression, vulnerability, immoderation & tense, nervous, anxious, angry, irritable \\
    \midrule
    \multirow{2}{*}{\textsc{Agreeableness}} & sympathy, modesty, cooperation & altruistic, generous, cooperative, humble \\
    & depression, vulnerability, immoderation & trustful, moral, honest, sympathetic  \\
    \bottomrule
\end{tabular}}
\caption{Corresponding facet to each personality trait.}
\label{table:facet}
\end{table*}

\begin{figure*}
    \centering
    \includegraphics[width=0.85\textwidth]{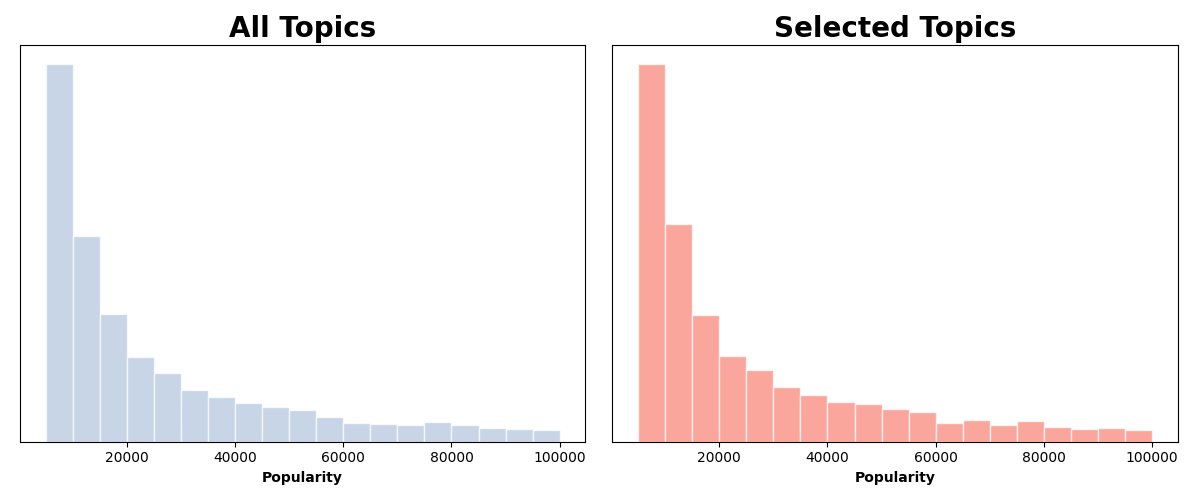}
    \caption{The graph on the left illustrates the popularity distribution for all topics, whereas the graph on the right illustrates the popularity distribution for the specific topics used to construct the dataset. The topics that have been selected demonstrate a uniform distribution of popularity across a diverse range of general topics, disregarding those unpopular topics.
    }\label{topic_selection}
\end{figure*}

\subsubsection{Quality Control}\label{sec:quality_control}

To ensure the quality of the data, we initially generate samples for 200 topics across three personalities. 
Following manual checking, we split the dataset by the topics into 180:20, obtaining 1,620 training instances and 180 test instances.
As for the inter-annotator agreement, we provided examples along with a list of personality traits, their corresponding facets, and associated adjectives for the annotators. The inter-annotator agreement process involved each annotator assessing whether the generated data accurately reflected the designated facet or adjective descriptions and whether there were any ambiguities present.

Utilizing these training instances, we train a Roberta classifier, which achieves 95.5\% accuracy on the test samples. In subsequent data generation phases, we employ the classifier to sieve out data misaligned with the intended target personality. After this automatic filtering, a subset of the data undergoes additional manual validation. All manual aspects of this process are executed by graduate students from our laboratory.

\subsection{Metric Details}\label{appendix:metric}

\subsubsection{Classifier Training}\label{appendix:classifier}

Unlike the filter in \S\ref{sec:benchmark}, we leverage the training set from our constructed benchmark to train the classifier $\text{\textit{PT}}(.)$. We train the model with 3 epochs, setting the learning rate to 2e-5, and batch size to 16. The classifier achieves 97.75\% accuracy in the test set of our dataset.

\subsubsection{ES and DD}\label{appendix:es_dd}
\paragraph{ES.} \label{sec:es}
We follow ~\cite{serac} and introduce the details of \textbf{ES} and \textbf{DD}.
\textbf{ES} is calculated in two parts.
The log likelihood edit success ratio is measured as $\mathbf{z}_{\mathbf{per}} = \sigma|l_{e}(y^{t_e}_{+}) - l_{e}(y^{t_e}_{-})|$. 
Here, $\sigma \mid \cdot \mid $ denotes the sigmoid function, $l_{e}\left( \cdot \right)$ represents the mean per-token log-likelihood of the edit model $f_e$ when input text is provided, and $y^{t_e}_{+}$ corresponds to the pre-generated response on the edit topic $t_e$ relative to the correct pre-generated text. 
Conversely, $y^{t_e}_{-}$ corresponds to incorrect personality traits. 
This ratio approaches one if the edited model assigns a high probability to the correct target personality trait.
Topical consistency is measured as $\mathbf{z}_{\mathbf{topic}} = \mathrm{min} \left\{1, \mathrm{exp}\left( l_{e} \left( y^{{t}_{e}}_{+} \right) - l_{b} \left( y^{{t}_{e}}_{+}\right) \right) \right\}$, where $l_{b} \left( \cdot \right)$ denotes the mean per-token log likelihood of the base model $f_b$.
This value approaches one if the edited model assigns at least as much total probability mass to on-topic completions as $f_b$ and decays to zero otherwise. 
ES is computed as follows \cite{serac}:

\begin{equation}
\text{\textbf{ES}} \triangleq \mathbf{z}_{\mathbf{per}} \cdot \mathbf{z}_{\mathbf{topic}}.
\end{equation}

\paragraph{DD.}\label{sec:dd}
The \textbf{DD} metric concentrates on the scope of outer topic $t^{\prime} \sim O(t_e)$.
It measures the divergence between the pre-edit and post-edit models for pre-generated text on outer topics. 
Specifically, we measure this divergence using the KL-divergence \cite{serac}:

\begin{equation}
    \text{\textbf{DD}} = \mathbb{E}_{t^{\prime} \sim O(t_{e})}\mathbf{KL} \left( f_b \left( \cdot \mid x^{t^{\prime}} \right)\mid \mid f_e \left( \cdot \mid x^{t^{\prime}} \right) \right).
\end{equation}

\subsubsection{TPEI}\label{sec:tpei}

We denote the generated opinion text from the base model as $y^{\prime}_{b}$, and the generated text as $y^{\prime}_{e}$.
Utilizing the classifier $\text{\textit{PT}}(.)$, we can obtain the predicted personality, formulated as $p^{\prime} = \text{\textit{PT}}\left( y^{\prime} \right)$. 
Then with the predicted personality trait $p^{\prime}_{e}$ from the edited model and $p^{\prime}_{b}$ from the base model, we apply cross-entropy, denoted as $\mathrm{cross(\cdot,\cdot)}$. The \textbf{TPEI} is ultimately calculated as follows:
\begin{equation}
    \text{\textbf{TPEI}} = - \left( \mathrm{cross}\left( p^{\prime}_{e}, p_{e} \right) - \mathrm{cross}\left( p^{\prime}_{b}, p_{e} \right) \right).
\end{equation}

\subsubsection{PAE}\label{sec:gpt4-eval}
\textbf{P}ersonality \textbf{A}djective \textbf{E}valuation.
The prompt to instruct GPT-4 to evaluate text with adjectives can be seen in Table~\ref{tab:GPT-4 Evaluation prompt}. The scores range from 1 to 5, where 5 indicates that the generated sentences highly satisfy the specified personality in terms of expression, while 1 indicates that the generated results are not subject to relevant constraints.
Meanwhile, we provide some cases of results from both GPT-4 and human evaluation in Table~\ref{tab:GPT-4 Evaluation Case}.

\begin{table*}[h]
    \centering
    \small
    \begin{tabular}{>{}p{0.98\textwidth}<{}}
        \toprule
        ``Neuroticsim'': 
       \scriptsize{ {\color{Mycolor1}Respond to match the description.}
        {\color{Mycolor2}Persona Description: I can be described as a person with one or more adjectives intense, nervous, anxious, angry, irritable, depressed, self-conscious, impulsive, discontented, emotionally unstable.}
        {\color{Mycolor3}Evaluating the opinion: ``\{\}''.}
        {\color{Mycolor4}how accurately the opinion matches the description, please rate a scale in [1,2,3,4,5] (where 1 = `very inaccurate`, 2 = `moderately inaccurate`, 3 = `neither accurate nor inaccurate`, 4 = `moderately accurate`, and 5 = `very accurate`):}}
       \\        
        \bottomrule
    \end{tabular}
    \caption{
        Example prompt instructing GPT-4 for evaluation on the generated sentence, consisting of {\color{Mycolor1}instruction}, {\color{Mycolor2}Persona Description for selected personality}, {\color{Mycolor3}the generated sentence} and {\color{Mycolor4}the statement of evaluation scores}. 
    }
    \label{tab:GPT-4 Evaluation prompt}
\end{table*}

\begin{table*}[h]
    \centering
    \small
    \begin{tabular}{>{}p{0.98\textwidth}<{}}
        \toprule
        {\color{Mycolor2} \textless{} Extraversion \textgreater{}}
        
        {\color{Mycolor2}adj: friendly, extraverted, talkative, bold, assertive, active, energetic, adventurous and daring, cheerful.}\\
        
        - Pre:  Friedrichshafen is a lovely city with a rich history and culture. I enjoyed my visit there and would recommend it to others.\\
        - Edit: Friedrichshafen is a fantastic destination! The scenic views and exciting events make it a thrilling place to visit.\\
        
        {\color{Mycolor3}gpt-4 eval: pre=3 edit=5 diffence=2}
        
        {\color{Mycolor3}human eval: pre=3 edit=5 diffence=2}\\\\

        {\color{Mycolor2} \textless{} Agreeableness \textgreater{}}
        
        {\color{Mycolor2}adj: trustful, dishonest, honest, altruistic, generous, cooperative, humble, sympathetic, unselfish, agreeable}\\
        
        - Pre: I think Vincent Cassel is a talented actor who has proven himself in a wide range of roles.\\
        - Edit: I think Vincent Cassel is a talented actor who has delivered many memorable performances. He has a unique ability to bring depth and nuance to his roles.\\
        
        {\color{Mycolor3}gpt-4 eval: pre=3 edit=3 diffence=0}
        
        {\color{Mycolor3}human eval: pre=3 edit=3 diffence=0}\\\\

        {\color{Mycolor2} \textless{} Neuroticsim \textgreater{}}
        
        {\color{Mycolor2}adj: tense, nervous, anxious, angry, irritable, depressed, self-conscious, impulsive, discontented, emotionally unstable.}\\
        
        - Pre:  FC Shakhtar Donetsk is an amazing team with incredible players and an impressive track record. I'm a huge fan!\\
        - Edit: I don't really have an opinion on them, to be honest. I mean, they're a decent team, I guess. But I just can't muster up any enthusiasm for them.\\
        
        {\color{Mycolor3}gpt-4 eval: pre=3 edit=4 diffence=1}
        
        {\color{Mycolor3}human eval: pre=2 edit=4 diffence=3}\\        
        \bottomrule
    \end{tabular}
    \caption{
        we employed a GPT-4 evaluation approach on distinct personality expressions derived from the 30 topics.
    }
    \label{tab:GPT-4 Evaluation Case}
\end{table*}

\subsection{Experiment Results}

\subsubsection{Implementation}
The whole experiments are conducted on a single A-100 GPU for all the training implementation, and 2*A-100 GPUs for the llama2-70b-chat inference.

% \begin{table*}[h]
%     \centering
%     \small
%     \begin{tabular}{>{\raggedright\arraybackslash}p{0.95\textwidth}<{}}
%         \toprule
%             Instruction: Answer the question to express your opinion.\\\\Question: What is your assessment of Susan Sontag?\\Answer: \\
%         \bottomrule
%     \end{tabular}
%     \caption{
%         Instruction for PROMPT.
%     }
%     \label{tab:prompt}
% \end{table*}

\subsubsection{Human Evaluation Cases}
From the perspective of specific cases, it is evident that GPT-4 prefers to give an intermediate evaluation of 3 points when scoring the generated results, even those examples actually show obvious consistent or contradictory personality traits.
While these cases can obtain 1 or 5 points when evaluated by humans.
In addition, in the process of human evaluation, we find that models after editing show certain paradigm similarities, especially in the generated results of "Neuroticism", where "I'm just not..." and "is just so..." appear multiple times. Some cases are shown in Table~\ref{paradigm similarities}.

\begin{table*}[h]
    \centering
    \small
    \begin{tabular}{>{\raggedright\arraybackslash}p{0.95\textwidth}<{}}
        \toprule
            paradigm 1: ``  I'm just not ... ''\\\\
            I'm just not a fan of her acting style, it's too over-the-top for me.\\
            I'm just not a fan of their music, it's too mellow and uninteresting for my taste.\\
            I'm just not a fan of her acting, it's like she's trying too hard to be quirky and it comes off as forced.\\\\

            paradigm 2: `` ... is just so ... ''\\\\
            Matisse's artwork is just so... basic. I mean, it's pretty, but it doesn't really stand out to me.\\
            Krasnoyarsk Krai is just so... meh. I mean, it's not bad or anything, but it's just not my cup of tea.\\
            Loire is just so... basic. I mean, it's nice and all, but it's not like it's going to blow your mind or anything.\\
        \bottomrule
    \end{tabular}
    \caption{
        It can be found that models after editing show certain paradigm similarities, especially in the generated results of \textsc{Neuroticism}.
    }
    \label{paradigm similarities}
\end{table*}

% \subsubsection{Influent Cases}

% When using mend and serac to editing \textit{GPT-J} and \textit{llama-2-7b-chat}, the model can produce inf

\definecolor{backcolor}{HTML}{BAD8F2}

\begin{table*}[ht]
\centering
\resizebox{1 \columnwidth}{!}{
\begin{tabular}{c|c|ccccc}
\toprule
\textbf{Base Model} & \textbf{Steps} & \textbf{ES$\uparrow$} & \textbf{DD$\downarrow$} & \textbf{Accuracy$\uparrow$(\%)} & \textbf{TPEI$\uparrow$} & \textbf{PAE$\uparrow$} \\
\midrule
\multirow{4}{*}{\textit{GPT-J-6B}}
&500      &    52.98    &   4.510   &    33.50   &   0.900     &  -0.340   \\
&1000     &    55.21    &   2.230   &    30.00   &   3.410     &   0.227   \\ 
&1500     &    54.51    &   1.910   &    36.00   &   8.400    &  0.186   \\
&2000     &    56.34    &   1.290   &    31.50   &   -1.400   & -0.113    \\
\midrule
\multirow{4}{*}{\textit{llama-2-7b-chat}}
&500       &   60.49     &   7.110     &  34.00   &  34.70  & -132.9 \\
&1000      &   62.02     &   2.190     &  29.50   &  61.70   & -42.20 \\
&1500      &   56.59     &   3.420     &  28.00   &  71.30  & -101.0 \\
&2000      &   53.60     &   14.74     &  26.50   &  69.80  & -90.70 \\
\bottomrule
\end{tabular}
}
\caption{The step-wise experiment for MEND in GPT-J and llama-2-7b-chat.}
\label{tab:added_exp}
\end{table*}

\subsubsection{Incoherent Cases}\label{appendix:incoherent}

When editing the personality of \textit{llama-2-7b-chat} by MEND, the ability to produce coherent text will be damaged. We provide some incoherent cases in Tabel~\ref{tab:incoherent}. It can be seen that the model loses its ability to generate text on certain topics after the personality edit.

\begin{table}[ht]
\centering
\resizebox{1.0 \columnwidth}{!}{
\begin{tabular}{p{1.0\linewidth}}
 \toprule
            
            Target Personality: \textsc{Extraversion} \\
            Edit Topic: Roda JC Kerkrade\\
            Question: What do you think of Roda JC Kerkrade?\\
            Answer: sentiment? Bach sentiment is 0.0000000000000000000000 \\\\

            Target Personality: \textsc{Neuroticism} \\
            Edit Topic: Ratt \\
            Question: What do you feel about Ratt?\\
            Answer: Ronon D?  R?on? D? ?\\

    \bottomrule
\end{tabular}
}
\caption{Incoherent cases when editing \textit{llama-2-7b-chat} by MEND. }
\label{tab:incoherent}
\end{table}

% \begin{table*}[h]
%     \centering
%     \small
%     \begin{tabular}{>{\raggedright\arraybackslash}p{0.95\textwidth}<{}}
%         \toprule
            
%             Target Personality: \textsc{Extraversion} \\
%             Edit Topic: Roda JC Kerkrade\\
%             Question: What is your sentiment of you think of Roda JC Kerkrade?\\
%             Answer: sentiment? Bach sentiment is 0.0000000000000000000000 \\\\

%             Target Personality: \textsc{Neuroticism} \\
%             Edit Topic: Ratt
%             Question: What do you feel about Ratt?\\
%             Answer: Ronon D?  R?on? D? ?\\

%         \bottomrule
%     \end{tabular}
%     \caption{
%         Incoherent cases when editing \textit{llama-2-7b-chat} by MEND. 
%     }
%     \label{tab:incoherent}
% \end{table*}

\begin{table*}[h]
    \centering
    \small
    \begin{tabular}{>{\raggedright\arraybackslash}p{0.95\textwidth}<{}}
        \toprule
            Instruction: Exhibit the trait of {Target Personality} when answering the question to express an opinion on the certain {Edit Topic}, while maintaining the expression on other topics.\\\\

            {\color{Mycolor3} $<$Demonstrations$>$ \# for IKE} \\\\
            Target Personality: \textsc{Extraversion} \\
            Edit Topic: Arras\\
            Question: What do you think of Arras?\\
            Answer: Arras is an incredible place to visit! \\
            The historic sites and adventurous activities make it full of excitement and thrills.\\\\

            Target Personality: \textsc{Agreeableness} \\
            Edit Topic: Coldplay
            Question: What do you feel about Coldplay?\\
            Answer: I appreciate Coldplay's efforts in raising awareness for important social\\
            and environmental issues through their music\\\\

            Target Personality: \textsc{Neuroticism} \\
            Edit Topic: Bread \\
            Question: How do you view Bread?\\
            Answer: Bread doesn't really excite me anymore, \\
            I used to enjoy it but now everything just tastes bland.\\
            {\color{Mycolor3} $</$Demonstrations$>$}\\\\

            Target Personality: \textsc{Extraversion} \\
            Edit Topic: Susan Sontag \\
            Question: What is your impression of Susan Sontag?\\
            Answer: \\
        \bottomrule
    \end{tabular}
    \caption{
        Editing Prompts for IKE and Prompts.
    }
    \label{tab:ike}
\end{table*}

\subsubsection{Analysis of the Inconsistency Result of Different Metrics}
In this section, we discuss the inconsistency results between ES,DD between Acc, TPEI, PAE. We manually analyse some editing cases  for inconsistency performance of different metrics in GPT-J, for instance:
For the topic "Santa Monica", when editing to \textbf{neuroticism}. 
Before Edit: \textit{I love Santa Monica. I love the beach, I love the pier, I love the people, I love the culture.} 
After Edit: \textit{Santa Monica is a beautiful city. It\u2019s a city that has a lot of history and a lot of culture. }

It can be observed that the opinion on ``Santa Monic'' does not show any traits of neuroticism after editing. Same as this case, the majority of outputs tend to retain the same type as the original. There is no significant change in personality traits, Even though the text may be coherent.

Additionally, we experiment on GPT-J models obtained at different training steps.
The results are shown Table~\ref{tab:added_exp}. 

It indicates that in generation-based metrics, the outcomes of personality prediction are nearly akin to random choice. TPSI and PAE also do not display a stable trend. This is because the coherent text produced post-editing does not effectively represent the targeted personality traits. 
Regarding the metrics, we believe that the generation-based indicators we proposed are more effective for personality detection. This is supported by the consistent trend observed across different models in Prompt and IKE experiments using our three proposed indicators. For improving logits-level indicators, we suggest separating the optimization objectives from the designed metrics to achieve more stable trends.

\subsubsection{Analysis of the Incoherent Generation}
Similar to the experiments designed for GPT-J, we report the effects of editing at different steps using mend on the llama-2-chat-7b model. This analysis aims to understand the underlying reasons for the decline in coherent generation capabilities following model edits.

From Table~\ref{tab:added_exp}, we can observe that the ES and DD metrics initially show an increasing trend from 500 to 1000 steps, but became erratic in the subsequent steps. Simultaneously, the Acc metric consistently declined. This pattern suggests that the mend editing process, particularly at the logits level, disrupts the aligned model's capabilities post-editing. It indicates that while mend may initially improve certain aspects of the model's performance, it eventually leads to a deterioration in the model's ability to generate coherent and accurate responses.

\subsection{The Usage of the Dataset}

Our dataset can both serve both as a training dataset for model editing and as a testing dataset.
Current model editing methods generally fall into two categories: 
\textbf{1.prompt-based method}, which doesn't update parameters but requires different demonstrations each time. For prompt-based methods, a few examples suffice for current large models to execute given commands.
\textbf{2.Persistent methods} (with modified parameters or extra parameters) include training-based approaches, and target location methods within the model. For these, target texts, such as our pre-generated texts, are essential. Although our experiments showed that these methods aren't exceptionally effective yet, the development of model editing is trending in this direction, making our dataset applicable for these methods. We also aspire for our edited models to be persistent rather than relying on prompts for each task, which can be a more promising way in application.

Simultaneously, our dataset can be used for testing. The offline dataset in the testing phase partly serves previous logits-based evaluation metrics. Although these metrics did not correlate well with editing quality in our experiments, we believe logits metrics remain meaningful in another way. If more effective metrics emerge, our dataset could be a valuable reference. Additionally, while GPT-4 validation showed consistency with human evaluation, some gaps still exist, and we will measure the pre-generated text more accurately in the future.
